# Supplementary material for: Energy-aware Joint Orchestration of 5G and Robots: Experimental Testbed and Field Validation
Source: arXiv:2503.19613 source file (2025-03-25)
Supplement: Supplementary file 1 [file appendix.tex]

\appendices
\section{Constraint \ref{eq:const9a} Linearization}
\label{sec:linearization}

Considering that $l_{r,t,a,b}$ is a binary variable, we need to linearize the multiplication $l_{r,t,a,b} \times l_{r,t+1,a',b'}$. We can define a new binary variable $\varUpsilon_{r,t+1,a,b,a',b'} = l_{r,t,a,b} \times l_{r,t+1,a',b'}$, and the previous expressions on Equation \ref{eq:const9a} can be reformulated as:

\begin{gather}
	\label{eq:const15}
	b_{r,t+1} = b_{r,t} +  CR \times  u_{r,t+1}  - P_{RX} \times (1 - u_{r,t+1}) - \notag \\ 
	\sum_{a \in A} 	\sum_{b \in B} 	\sum_{a' \in A} \sum_{b' \in B}  \varUpsilon_{r,t+1,a,b,a',b'}  \times  P_{move_{a,b,a',b'}}   \notag \\ 
	- P_{SEN}  \times  \sum_{a \in A} 	\sum_{b \in B} (1 - e_{t,a,b}) \times l_{r,t+1,a,b} -  \\ 
	\sum_{a \in A} 	\sum_{b \in B}  P_{TX,a,b} \times (1 - e_{t,a,b}) \times l_{r,t,a,b} \quad \forall t \in \mathcal{T} , \forall r \in \mathcal{R}   \notag
\end{gather}
with the variable $\varUpsilon_{r,t+1,a,b,a',b'} $ fulfilling the following restrictions:

\begin{gather}
	\varUpsilon_{r,t+1,a,b,a',b'} \leq l_{r,t,a,b} \quad \notag \\ 
	\forall r \in \mathcal{R} , \forall t \in \mathcal{T}, \forall (a,b) \in (A,B), \forall (a',b') \in (A,B)
	\label{eq:const9.1}
\end{gather}

\begin{gather}
	\varUpsilon_{r,t+1,a,b,a',b'} \leq l_{r,t+1,a',b'} \quad \notag \\ 
	\forall r \in \mathcal{R} , \forall t \in \mathcal{T}, \forall (a,b) \in (A,B), \forall (a',b') \in (A,B)
	\label{eq:const9.2}
\end{gather}

\begin{gather}
	\varUpsilon_{r,t+1,a,b,a',b'} \geq l_{r,t,a,b} + l_{r,t+1,a',b'} - 1 \quad \notag \\
	\forall r \in \mathcal{R} , \forall t \in \mathcal{T}, \forall (a,b) \in (A,B), \forall (a',b') \in (A,B)
		\label{eq:const9.3}
\end{gather}

But we can also reduce the number of variables as there are only some possible situations according to Equations \ref{eq:const7} and \ref{eq:const8}, therefore:

\begin{gather}
	\varUpsilon_{r,t+1,a,b,a',b'} = 0 \quad  \forall r \in \mathcal{R} , \forall t \in \mathcal{T}  	\label{eq:const9.4} \\
	\text{if } a-1 > a' > a+1 \text{ or if } b-1 > b' > b+1 , \notag 
\end{gather}

\begin{comment}
We can also linearize the multiplication $u_{r,t} \times l_{r,t,a,b}$ by defining a new binary variable $\delta_{r,t,a,b} = u_{r,t} \times l_{r,t,a,b}$, where the new variable needs to fulfill the following constraints:

\begin{gather}
	\label{eq:const9.5}
	\delta_{r,t,a,b} \leq u_{r,t} \quad	\forall r \in \mathcal{R} , \forall t \in \mathcal{T}, \forall (a,b) \in (A,B)
\end{gather}

\begin{gather}
	\label{eq:const9.6}
	\delta_{r,t,a,b} \leq l_{r,t,a,b} \quad	\forall r \in \mathcal{R} , \forall t \in \mathcal{T}, \forall (a,b) \in (A,B)
\end{gather}

\begin{gather}
	\label{eq:const9.7}
		\delta_{r,t,a,b} \geq u_{r,t} + l_{r,t,a,b} - 1 \quad \notag \\
	\forall r \in \mathcal{R} , \forall t \in \mathcal{T}, \forall (a,b) \in (A,B)
\end{gather}
\end{comment}

We can linearize the multiplication $e_{t,a,b} \times l_{r,t+1,a,b}$ by defining a new binary variable $\alpha_{r,t,a,b} = e_{t,a,b} \times l_{r,t+1,a,b}$, where the new variable needs to fulfill the following constraints:
%Finally, we can also introduce the new binary variable $\alpha_{r,t,a,b} = e_{t,a,b} \times l_{r,t,a,b}$, and the following constraints:

\begin{gather}
	\label{eq:const9.8}
	\alpha_{r,t,a,b} \leq e_{t,a,b} \quad	\forall r \in \mathcal{R} , \forall t \in \mathcal{T}, \forall (a,b) \in (A,B)
\end{gather}

\begin{gather}
	\alpha_{r,t,a,b} \leq l_{r,t+1,a,b} \quad	\forall r \in \mathcal{R} , \forall t \in \mathcal{T}, \forall (a,b) \in (A,B)
	\label{eq:const9.9}
\end{gather}

\begin{gather}
		\alpha_{r,t,a,b} \geq e_{t,a,b} + l_{r,t+1,a,b} - 1 \quad \notag \\
	\forall r \in \mathcal{R} , \forall t \in \mathcal{T}, \forall (a,b) \in (A,B) 
	\label{eq:const9.10}
\end{gather}

And Equation \ref{eq:const9a} can be finally reformulated as:

\begin{gather}
	\label{eq:const9}
	b_{r,t+1} - b_{r,t} 	+ \sum_{a \in A} 	\sum_{b \in B} l_{r,t+1,a,b} \times (P_{TX,a,b} + P_{SEN})  \notag \\ 
	+  	\sum_{a \in A} 	\sum_{b \in B} 	\sum_{a' \in A} \sum_{b' \in B}  \varUpsilon_{r,t+1,a,b,a',b'}  \times P_{move_{a,b,a',b'}}   \notag \\ 
 -  \sum_{a \in A} 	\sum_{b \in B} \alpha_{r,t,a,b} \times (P_{TX,a,b} + P_{SEN})   \notag \\ 
	- u_{r,t+1} (CR + P_{RX} ) = - P_{RX}   \quad \forall t \in \mathcal{T} , \forall r \in \mathcal{R}   
\end{gather}

\section{Constraint \ref{eq:const20} Linearization}
\label{sec:linearizationB}

Again, considering that $l_{r,t,a,b}$ is a binary variable, we need to linearize the multiplication $l_{r,t,a,b} \times l_{r,t+1,a',b'}$. We can define a new binary variable $\varUpsilon_{r,t+1,a,b,a',b'} = l_{r,t,a,b} \times l_{r,t+1,a',b'}$. 
We can also linearize the multiplication $u_{r,t+} \times l_{r,t+1,a,b}$ by defining a new binary variable $\delta_{r,t,a,b} = u_{r,t} \times l_{r,t,a,b}$. Now, Equation \ref{eq:const20} can be reformulated as:

\begin{gather}
	b_{r,t+1} = b_{r,t} +  (CR + P_{RX} + P_{SEN}) \times  u_{r,t+1} - P_{RX} - P_{SEN} \notag \\ 
	-  \sum_{a \in A} 	\sum_{b \in B} 	\sum_{a' \in A} \sum_{b' \in B} \varUpsilon_{r,t+1,a,b,a',b'}  \times  P_{move_{a,b,a',b'}}  \notag \\ 
		+  \sum_{a \in A} 	\sum_{b \in B} P_{TX,a,b} \times  \delta_{r,t+1,a,b} 	 \notag \\ 
   -  \sum_{a \in A} 	\sum_{b \in B} P_{TX,a,b} \times l_{r,t+1,a,b} \quad \forall t \in \mathcal{T} , \forall r \in \mathcal{R} 
	\label{eq:const22}
\end{gather}
with $\varUpsilon_{r,t+1,a,b,a',b'}$ fulfilling Equations \ref{eq:const9.1}, \ref{eq:const9.2}, \ref{eq:const9.3} and \ref{eq:const9.4}, and where the new variable $\delta_{r,t,a,b}$ needs to fulfill the following constraints:

\begin{gather}
	\label{eq:const9.5}
	\delta_{r,t,a,b} \leq u_{r,t} \quad	\forall r \in \mathcal{R} , \forall t \in \mathcal{T}, \forall (a,b) \in (A,B)
\end{gather}

\begin{gather}
	\label{eq:const9.6}
	\delta_{r,t,a,b} \leq l_{r,t,a,b} \quad	\forall r \in \mathcal{R} , \forall t \in \mathcal{T}, \forall (a,b) \in (A,B)
\end{gather}

\begin{gather}
	\label{eq:const9.7}
		\delta_{r,t,a,b} \geq u_{r,t} + l_{r,t,a,b} - 1 \quad 	\forall r \in \mathcal{R} , \forall t \in \mathcal{T}, \forall (a,b) \in (A,B)
\end{gather}
